# Supplementary material for: Graph Matching Networks for Learning the Similarity of Graph Structured Objects
Source: arXiv:1904.12787 source file (2019-05-12)
Supplement: Supplementary file 1 [file appendix.tex]

\documentclass{article}
\usepackage[utf8]{inputenc}

\usepackage{nips_2018}

\usepackage[utf8]{inputenc} %
\usepackage[T1]{fontenc}    %
\usepackage{hyperref}       %
\usepackage{url}            %
\usepackage{booktabs}       %
\usepackage{amsfonts}       %
\usepackage{nicefrac}       %
\usepackage{microtype}      %
\usepackage{color}
\usepackage{symbols}
\usepackage{graphicx}
\usepackage{multirow}

\newcommand{\ignore}[1]{}

\title{Appendix for Deep Graph Similarity Learning}

\author{
  David S.~Hippocampus\thanks{Use footnote for providing further
    information about author (webpage, alternative
    address)---\emph{not} for acknowledging funding agencies.} \\
  Department of Computer Science\\
  Cranberry-Lemon University\\
  Pittsburgh, PA 15213 \\
  \texttt{hippo@cs.cranberry-lemon.edu} \\
}

\begin{document}

\maketitle

\input{appendix_content}

\bibliography{refs}
\bibliographystyle{plain}

\end{document}
